# Supplementary material for: DPE: Disentanglement of Pose and Expression for General Video Portrait Editing
Source: arXiv:2301.06281 source file (2023-03-01)
Supplement: Supplementary file 1 [file 12_appendix.tex]

\appendix
\label{sec:appendix}

% \section{}
\section{Additional Network Details}
\subsection{Motion Editing Module.} 
Our motion editing module consists of an encoder and several multiple perceptron (MLP) layers.
The encoder consists of a convolution layer followed by seven residual blocks with resolutions from 256 to 4. 
And the outputs of the first five residual blocks are viewed as part of $\mathcal{F}$ described in Sec.~\ref{sec:method}.
At the end of encoder, an additional convolution layer is used to project the feature maps to a latent space that is supposed to be decomposable into two orthogonal subspaces.
Based on the latent code, several MLP layers are used to disentangle the latent space of the encoder to two orthogonal subspaces.
Specifically, the architecture of the disentanglement module is that the first five MLP layers act as the shared backbone, followed by two heads that each consists of three MLP layers to decouple the expression and pose motion code, respectively.

\begin{figure}[t]
    \centering
    \includegraphics[width=\linewidth]{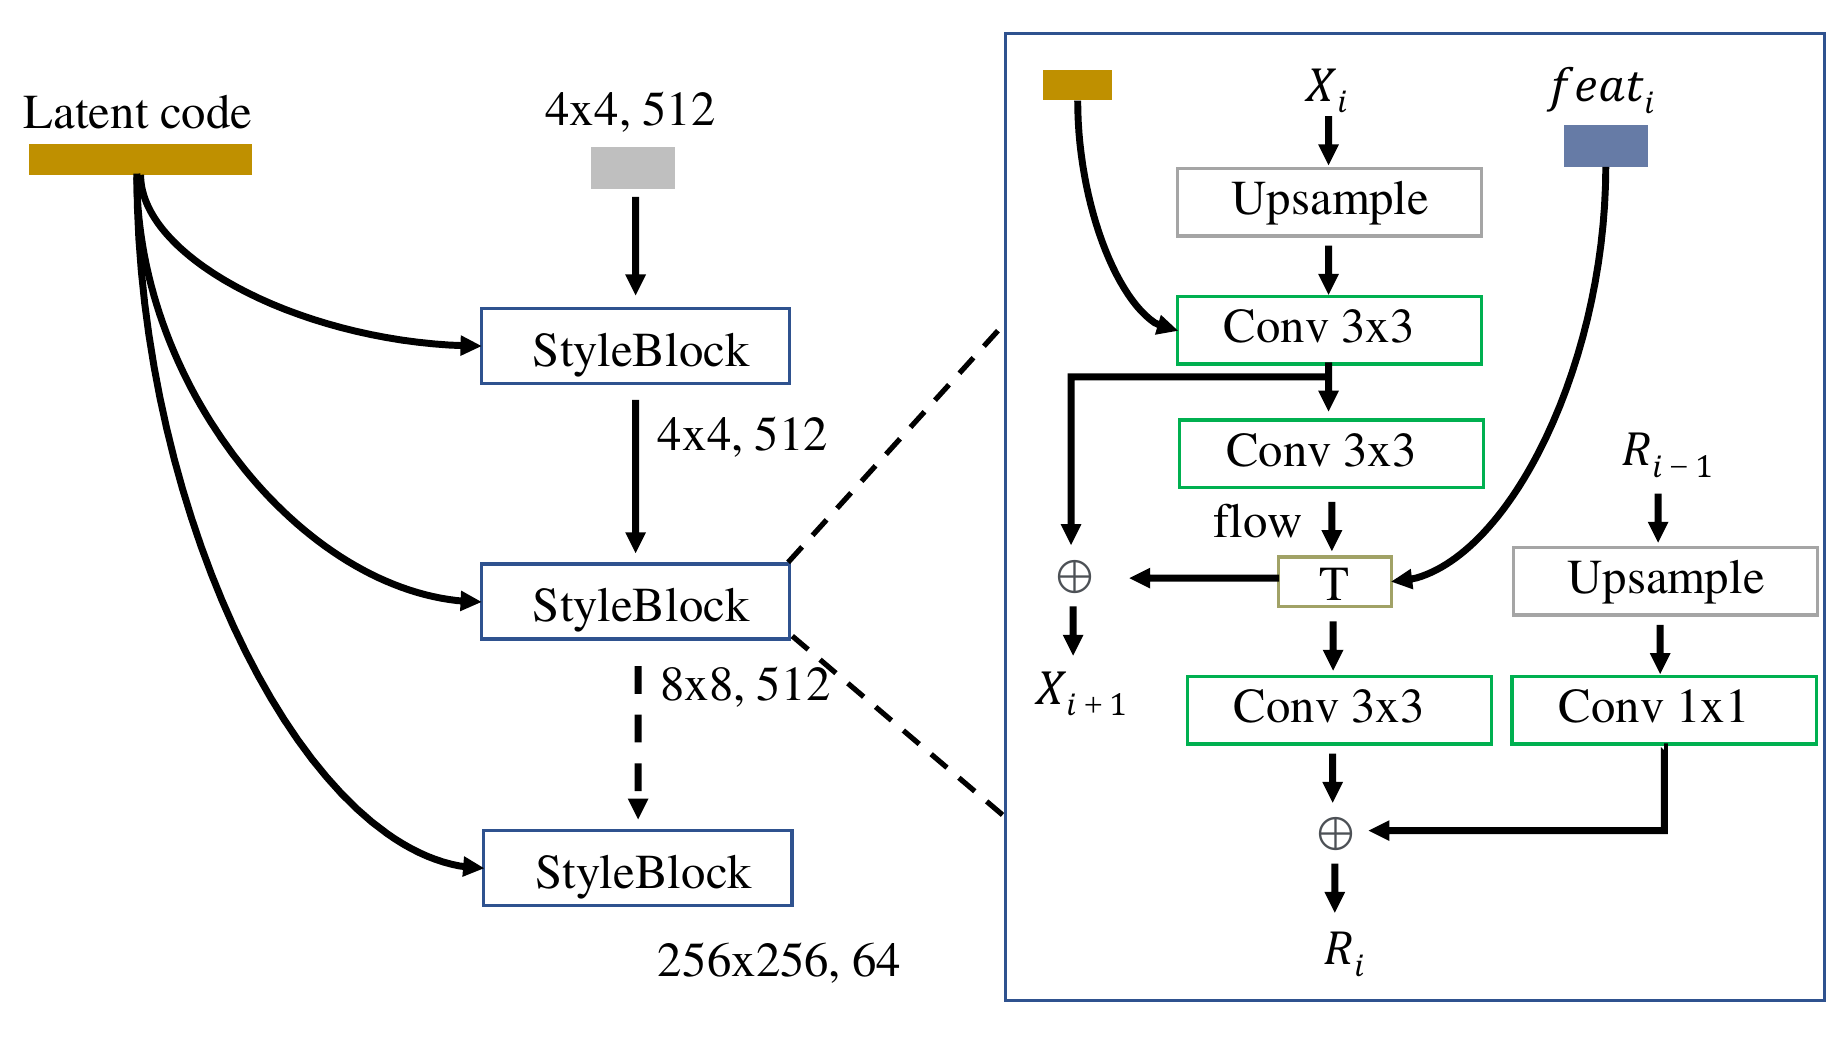}
    \caption{Pose and expression generators, which are based on StyleGAN2\cite{karras2020analyzing}. $T$ is the warping transformation. $R$ means RGB images. And $X$ indicates the output of each StyleBlock. }
    \label{fig:generator}
\end{figure}

\subsection{Pose and Expression Generators.}
The two generators share the same architecture but different parameters.
As shown in Fig.~\ref{fig:generator}, based on StyleGAN2\cite{karras2020analyzing}, we exploit the latent code to generate multiscale flow fields that are used to warp the feature maps from the encoder in the motion editing module.
Specifically, StyleBlock from StyleGANS is borrowed to implement the whole process. 
There are two outputs in StyleBlock, one is the warped feature maps $X_{i+1}$, and the other is the RGB image $R_{i}$ with the current resolution. The inputs include $R_{i-1}$ and $X_{i}$ from the previous layer as well as latent code and feature maps from motion editing module. Each StyleBlock is used to upsample ×2 the previous resolution. We stack 6 blocks towards producing 256 resolution images.

\begin{figure}[t]
    \centering
    \includegraphics[width=\linewidth]{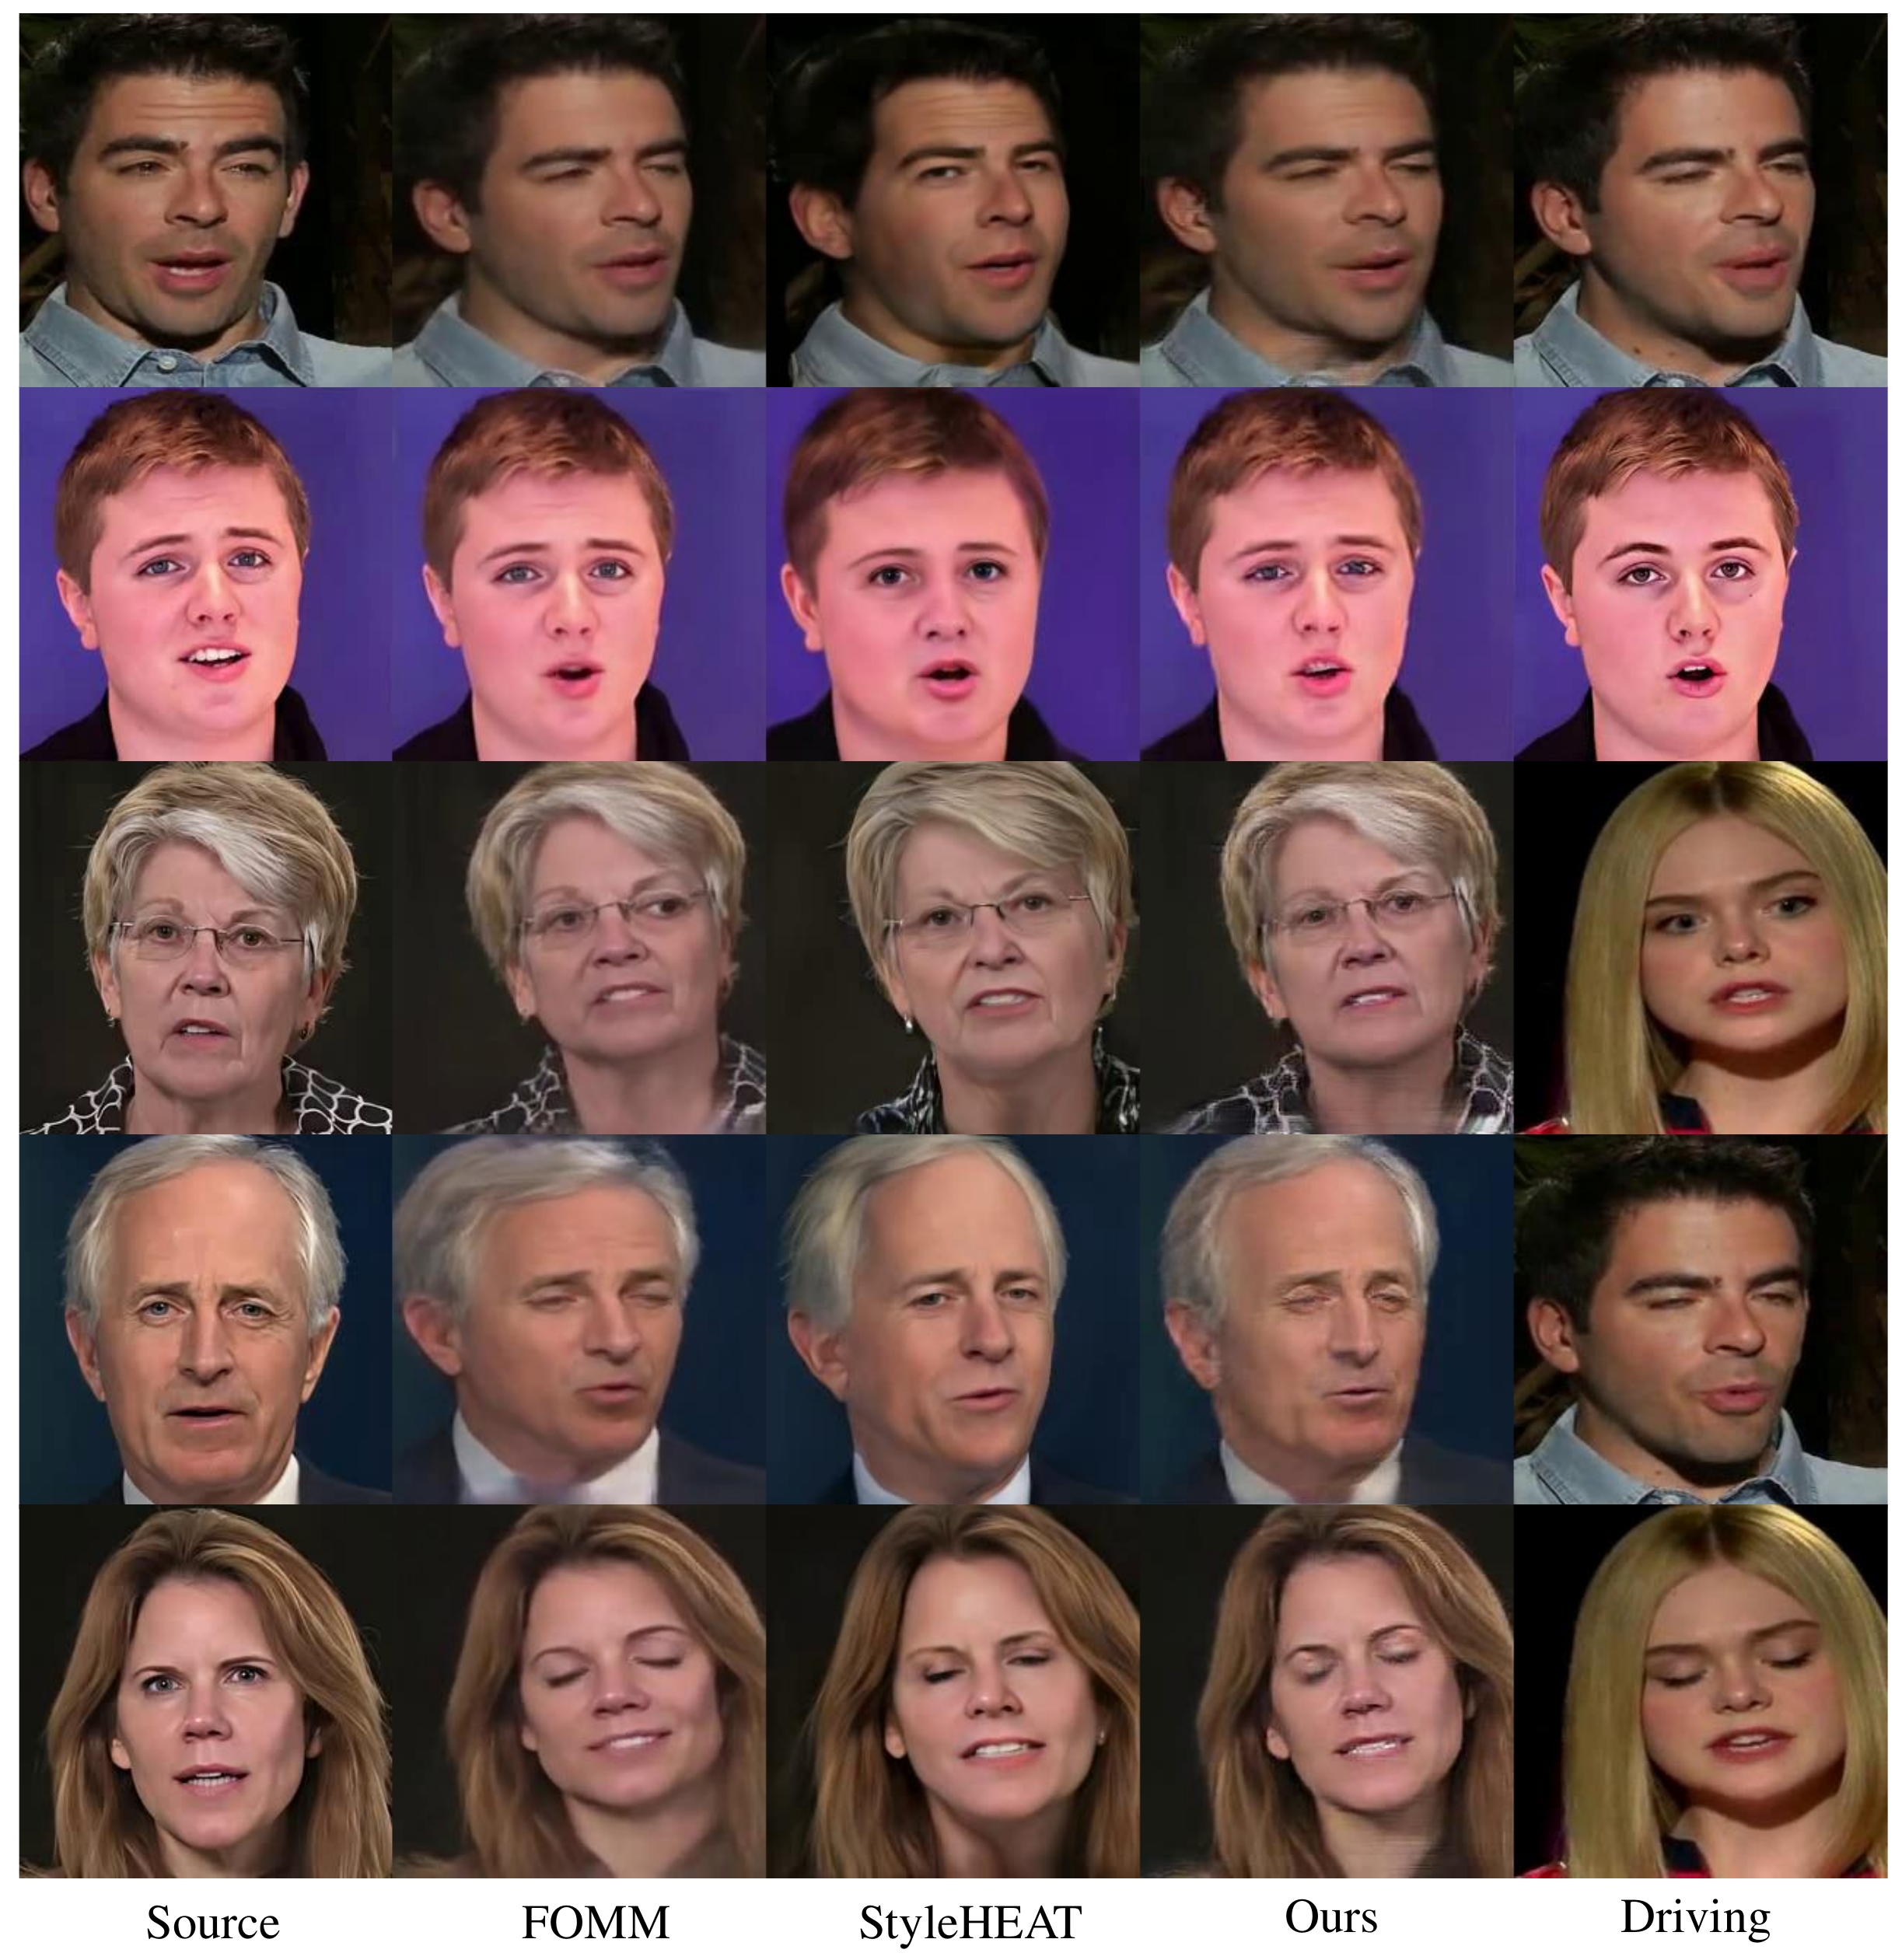}
    \caption{Comparisons with FOMM\cite{Siarohin_2019_NeurIPS} and StyleHEAT\cite{2203.04036} on one-shot talking face generation.}
    \label{fig:one}
\end{figure}

\section{Additional Experiment Details.}
In $video.mp4$, we compare with state-of-the-art methods on one-shot talking face generation and video portrait editing.
\subsection{One-shot Talking Face Generation.}
Due to space limitations in the main paper, we show the qualitative comparisons for FOMM\cite{Siarohin_2019_NeurIPS} and StyleHEAT\cite{2203.04036}.
According to Fig.~\ref{fig:one}, our method preserves the identity better than other two methods.
It can be observed that FOMM and StyleHEAT tend to change the face shape of the source image if the face shape of the driving image differs from the source. 
Especially for cross-identity reenactment, the face shape of FOMM is far away from the source face.
And FOMM produces twisted faces especially when the head pose difference is large between the source and driving faces.
Moreover, our method has better control over the details of expression. 
For same-identity reenactment, StyleHEAT is inaccurate about the handling of the eyes. 
For instance, as shown in the first row, the eye gaze is abnormal.
Also, in the forth row, StyleHEAT is not accurate for opening and closing of the eyes.

\subsection{Disentanglement for Video Portrait Editing.}
\begin{figure*}[t]
    \centering
    \includegraphics[width=\linewidth]{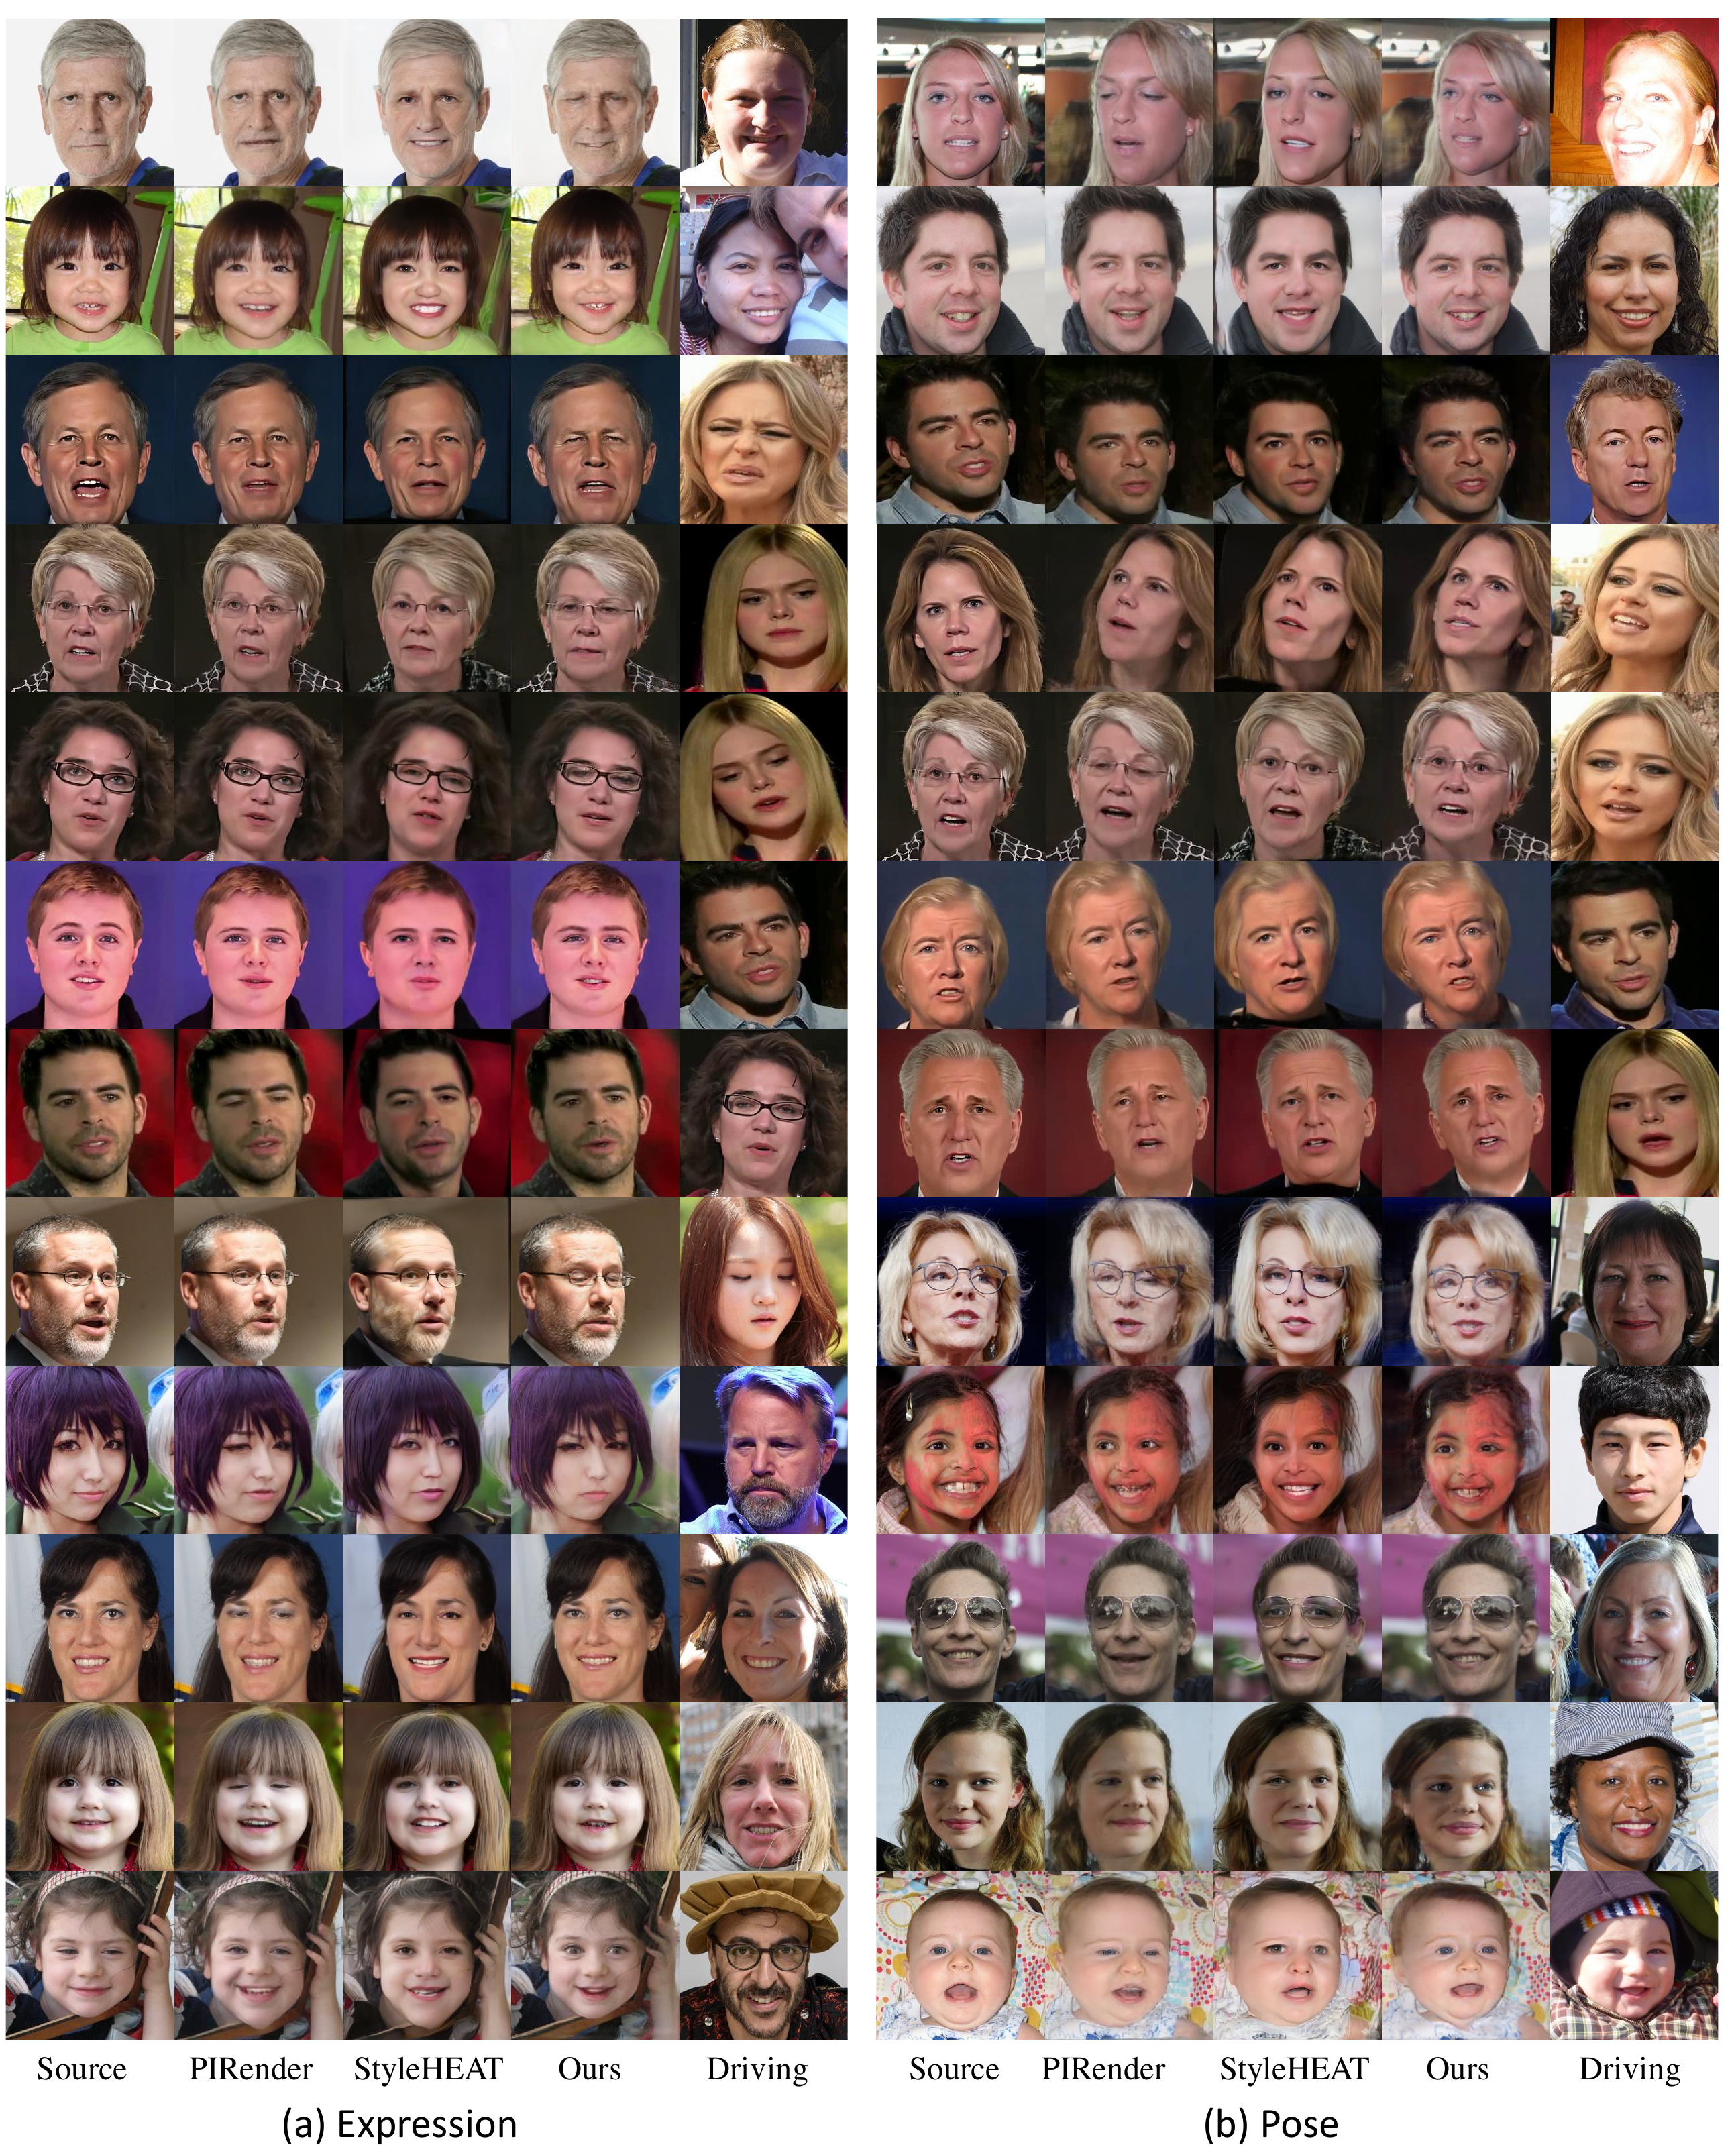}
    \caption{Comparisons with PIRender\cite{ren2021pirenderer} and StyleHEAT\cite{2203.04036} on disentanglement for video portrait editing.}
    \label{fig:dec}
\end{figure*}
For video demo, we download videos of real movies and news scenes from YouTube. 
Since the appropriate talking clips cannot be kept for a long time in movie scene when they are used as the source videos, we repeat them for a sufficient length of time to show the effect better.
As shown in $video.mp4$, we demonstrate the qualitative comparisons for PIRender\cite{ren2021pirenderer} and StyleHEAT\cite{2203.04036} by exchanging their 3DMM parameters for expression editing only.
For StyleHEAT, as the input face needs to be aligned, it cannot be directly pasted back to the original image.  So the whole face is shaking a lot.
For both PIRender and our method, faces move freely within a fixed bounding box and no need to align, so the results are better than StyleHEAT.
However, PIRender does not maintain the shape and identity of the source face well, as well as the transfer of the expression.
According to the red arrow of the videos, it can be seen that there is an obvious double-face phenomenon at the paste edge in PIRender.
In addition, there is also an obvious incongruity between the inner and outer faces of PIRender.
For instance, the inner face generated by PIRender is always swaying back and forth, but the hair and background are stable.
In contrast, our results are more stable and have better edge details.
In addition, PIRender is not accurate for the transfer of expression, especially for the eyes and mouths.
The reason is that the extracted 3DMM parameters by a pre-trained network cannot accurately reflect the status of eyes and mouth due to the limited number of Blendshapes.
Our method has yielded the best results.

In Fig.~\ref{fig:dec}, we demonstrate the qualitative comparisons for PIRender\cite{ren2021pirenderer} and StyleHEAT\cite{2203.04036}. 
It can be observed that PIRender and StyleHEAT tend to change the face shape of the source image if the face shape of the driving image differs from the source. 
And our method achieves better accuracy in expression transfer than the other two methods, especially the eyes and the mouth shape.

% \subsection{Audio-driven Video Portrait Editing.}
